# Supplementary material for: H2:Towards Efficient Large-Scale LLM Training on Hyper-Heterogeneous Cluster over 1,000 Chips
Source: arXiv:2505.17548 source file (2025-05-23)
Supplement: Supplementary file 1 [file appendix.tex]

\section{Appendix}

\begin{algorithm}[H]
\footnotesize                   
\setstretch{1.0}               
\caption{HeteroPP Automatic Parallel Strategy Search}
\label{alg:heteropp_search}
\begin{algorithmic}[1]
\Require  
\begin{itemize}[leftmargin=*,noitemsep]
  \item Set of chip types: for each chip type $i$, available chips $N_i$, safe memory $M_i$, maximum TP size $TP\_MAX_i$.
  \item Global mini-batch size $B$.
  \item Total number of neural network layers $L$.
  \item Tables:
    \begin{itemize}[leftmargin=*,noitemsep]
      \item Layerwise compute time per sample: $t_{\text{compute}}(i,\#TP_i)$.
      \item Layerwise optimizer step time: $t_{\text{step}}(i,\#DP,\#TP_i)$.
      \item Layerwise activation memory per sample: $mem_{act}(\#TP)$.
      \item Layerwise model\&optimizer states memory: $mem_{model}(\#DP, \#TP)$.
    \end{itemize}
  \item Pipeline overhead $t_{\text{loss}}$ and bubble coefficient $\alpha$.
\end{itemize}

\Statex
\textbf{Ensure: Optimal configuration:}
\begin{itemize}[leftmargin=*,noitemsep]
  \item Global data parallel size $\#DP$, micro-batch count $n_{mb}$.
  \item For each chip type $i$: number of PP stages $\#PP_i$, TP size $\#TP_i$, and number of layers per PP stage $L_i$.
\end{itemize}

\State $\mathbf{bestT} \gets \infty$
\State $\mathbf{bestConfig} \gets nil$

\LeftComment{Step 1: Enumerate candidate global DP sizes}
\For{each candidate $\#DP$ that divides $B$ evenly}
    \State $n_{mb} \gets \dfrac{B}{\#DP}$
    
    \LeftComment{Step 2: Enumerate feasible $(\#PP_i, \#TP_i)$ pairs for each chip type}
    \For{each chip type $i$}
        \State $\text{FC}_i \gets \emptyset$
        \For{each candidate $\#TP_i \in \{1, 2, 4, \dots, TP\_MAX_i\}$}
            \State Compute $\#PP_i \gets \dfrac{N_i}{\#TP_i \times \#DP}$
            \State Add Feasible $(\#PP_i,\, \#TP_i)$ to $\text{FC}_i$
        \EndFor
    \EndFor
    
    \State $\mathcal{C} \gets \{ (\#DP, n_{mb}, \{ (\#PP_i, \#TP_i) \}_{i} ) \;|\; (\#PP_i, \#TP_i) \in \text{FC}_i,\, \forall i \}$
    
    \LeftComment{Step 3: Search for optimal layer sharding}
    \For{$\mathcal{C}_c = (\#DP, n_{mb}, \{ (\#PP_i, \#TP_i) \}_{i}) \in \mathcal{C}$}
        \State Determine optimal layer division $\{L_i\}$ for each chip type $i$
        \If{the $\{L_i\}$ violates memory constraints Equation \ref{eq:pr6}}
            \State \textbf{continue}
        \EndIf

        \State
        \LeftComment{Step 4: Estimate iteration time components for the candidate}
        \State Calculate estimated iteration time cost $T$ by Equation \ref{eq:itertime}
        
        \If{$T < \mathbf{bestT}$}
            \State $\mathbf{bestT} \gets T$
            \State $\mathbf{bestConfig} \gets (\#DP, n_{mb}, \{ (\#PP_i, \#TP_i, L_i) \}_{i})$
        \EndIf
    \EndFor
\EndFor
\State \Return $\mathbf{bestConfig}$
\end{algorithmic}
\end{algorithm}
